# Supplementary material for: Dynamics as Prompts: In-Context Learning for Sim-to-Real System Identifications
Source: arXiv:2410.20357 source file (2025-02-28)
Supplement: Supplementary file 2 [file main.tex]

\documentclass[10pt]{article}
\usepackage[utf8]{inputenc}
\usepackage{amsmath}
\usepackage{amssymb}
\usepackage{xcolor}
\usepackage{geometry}
\geometry{a4paper, margin=1in}
\usepackage{enumitem}
\usepackage{cite} % For citations
\usepackage{graphicx}
\usepackage{algorithm}
\usepackage{algpseudocode}
\usepackage{hyperref}

% \usepackage{algcompatible}
% \usepackage{algorithmic}

% Custom commands for responses
\newcommand{\authorresponse}[1]{\textcolor{black}{\textbf{Author Response:} #1}}
\newcommand{\reviewercomment}[1]{\textcolor{blue}{\textbf{Reviewer Comment:} #1}}

\title{Dynamics as Prompts: In-Context Learning for Sim-to-Real System Identifications \#24-3480}
\author{Xilun Zhang*, Shiqi Liu*, Peide Huang, William Han, Yiqi Lyu, Mengdi Xu, Ding Zhao}
\date{}

\begin{document}

\maketitle

% General Comments Section

\section*{General Comments}

Thank you all for the constructive feedback and encouraging review. We appreciate that the reviewers find our proposed method CAPTURE novel and interesting. In addition to the detailed comments to each review, we would like to highlight our main modifications in the revision, including clarifications and additional experiments. We also highlighted the changes in red in the revised paper.
\begin{enumerate}
    \item \textbf{Additional experiments with different sequence length $K$ (Reviewer 1, Reviewer 3):} We conducted extensive ablation studies in \hyperref[sec:exp_1]{Experiment 1} by varying the sequence length $K$ for parameter transition iteration generation. The results confirm that the choice of $K$ within a reasonable range (e.g., 7 to 9) does not significantly affect system identification performance. This demonstrates that our proposed method is robust against the choice of sequence length.

    \item \textbf{Additional experiments with different window size $k$ (Reviewer 3):} We evaluated various window sizes $k$ for the SysID transformer in \hyperref[sec:exp_2]{Experiment 2} and observed that smaller window sizes lead to more stable and generalizable performance. The choice of variable $k$ can be task-dependent, as a more complex dynamic environment needs more histories to infer the correct environment parameters.

    \item \textbf{Justification of the ``over-fitting" behavior in table air hockey (Reviewer 3, Reviewer 5):} We clarified the observed performance trends in the table air hockey task. The slight increase in parameter estimation error after a certain iteration is attributed to Out-of-Distribution (OOD) conditions not encountered during training. Our experiments show that CAPTURE remains more robust in these OOD settings compared to baseline and ablation methods, highlighting its strong generalization capabilities.

    \item \textbf{Generalization to multi-task settings and related assumptions (Reviewer 2, Reviewer 5):} 
    % We discussed the feasibility of extending our approach to multi-task scenarios. 
    In this paper, we only focus on dynamics adaptation (environment parameter identifications) in specific tasks, where the tasks share the same state representation, action space, and environment parameter space. Multi-task learning would be a promising future direction in which to expand on current work.

    \item \textbf{Experiments with more recent baselines (Reviewer 2, Reviewer 5):} In response to reviewer feedback, we included the COMPASS at \hyperref[sec:exp_3]{Experiment 3} as an additional baseline from CoRL 2023. Our results show that CAPTURE outperforms COMPASS on both table air hockey and object scooping tasks in sim-to-sim evaluations. This comparison solidifies CAPTURE’s advantage over more recent and state-of-the-art approaches.
\end{enumerate}


% Reviewer 1
\section*{Response to Reviewer 1}
Thank you for your constructive feedback. We are pleased to hear that you found our work novel and compelling. Please find our detailed responses below.

\begin{enumerate}[label=\textbf{Q\arabic*.}, leftmargin=1.5cm]
    \item \reviewercomment{It would be clear if the task-specific training requirement was stated explicitly in the methodology.}    
    
    \authorresponse{We added the essential requirements at the beginning of section III of the revised paper, including assumptions, history components, and task-related information.}

    \item \reviewercomment{Some more architectural details on the transformer network.}    
    
    \authorresponse{We updated Section III-D in the revised paper to include an architectural description: To model sequential relations, we utilized the Decision Transformer [1] architecture, which incorporates GPT-2 [2] as the transformer backbone. This design facilitates the effective integration of historical trajectories and action sequences, enabling accurate environment parameter estimation.}
    
    \item \reviewercomment{Including an examination of the impact of different K values.}    
    
    \authorresponse{We expanded our analysis to include the impact of different sequence lengths $K$ and transformer window sizes $k$ in the additional experiments section. The results of the ablation study on $K$ values are detailed and discussed in \hyperref[sec:exp_1]{Experiment 1}, while the ablations on the transformer window size ($k$, history length during inference) are presented in \hyperref[sec:exp_2]{Experiment 2}. Our findings suggest that $K$ minimally impacts performance within the reasonable range of 7 to 9.}
\end{enumerate}

% Add References Between Reviewer 1 and Reviewer 2
\section*{References}
\begin{enumerate}[label=\textbf{\arabic*.}, leftmargin=1.5cm]
    \item Lili Chen, et al. ``Decision Transformer: Reinforcement Learning via Sequence Modeling'', 2021 Neural Information Processing Systems, 2021.
    \item Alec Radford, et al. ``Language Models are Unsupervised Multitask Learners'', OpenAI Technical Report, 2019.
\end{enumerate}

% Reviewer 2
\section*{Response to Reviewer 2}
Thanks for your thorough review of the article and showing interest in our experiments in both the simulation and the real world. We made the corresponding improvements to the paper and addressed your concerns below.

\begin{enumerate}[label=\textbf{Q\arabic*.}, leftmargin=1.5cm]
    \item \reviewercomment{The presentation deserves some improvement.} 
    
    \authorresponse{We revised the paper and improved the language for clarity and readability. The updated content is marked in red in the revised version. We hope these changes make the content clearer and easier to follow.
}
    
    \item \reviewercomment{Need more recent baselines.}    
    
    \authorresponse{We included the COMPASS[1] baseline in the additional \hyperref[sec:exp_3]{Experiment 3}. Our comprehensive sim-to-sim evaluations reveal that COMPASS does not achieve the same level of performance as CAPTURE in estimating environment parameters for both the table air hockey and object scooping tasks.}

    \item \reviewercomment{Justification on the parameter space being finite and bounded assumption.}  
    
    \authorresponse{In the real world, the physical parameters we considered are generally bounded. For instance, friction coefficients typically range between 0 and 1, and damping ratios for most mechanical systems remain within a finite range depending on the material properties and design. These bounded ranges are consistent with the environment parameters used in our simulations. Simulators typically provide a fixed number of tunable parameters with predefined ranges. While this assumption may simplify real-world dynamics, we assume that the range of environment parameters is large enough to reflect real-world behaviors. This property is supported by the COMPASS [1] paper, where they experimented with over 100 environment parameters, showing that these ranges are sufficient to capture diverse real-world dynamics. Additionally, the specific parameter ranges we selected are designed to cover and match the general behavior of real-world systems effectively.}

    \item \reviewercomment{Using task policy for trajectory generation.}    
    
    \authorresponse{While random actions offer broader exploration, task policies are more efficient for collecting task-specific data. In our approach, task policies prioritize task-relevant environment parameters, enhancing data efficiency in simulation. The rationale behind this choice has been included in the revised paper.}

    \item \reviewercomment{Potential fits on multi-task settings.} 
    
    \authorresponse{In the real-world object scooping experiments, we successfully demonstrated the ability to scoop different objects using a single SysID model. Expanding this capability to a multi-task setting—such as enabling the model to perform both object scooping and table air hockey—is feasible within our proposed framework by incorporating a higher-dimensional environment parameter space and more generalized state representations. In this paper, our focus is on dynamics adaptation (environment parameter identification) for specific tasks that share the same state representation, action space, and environment parameter space. We sincerely appreciate the suggestion, as multi-task learning represents an exciting and promising direction for future exploration.}
    
    \item \reviewercomment{Justify the advantage of smoother adaptation curves over less smooth methods.}
    
    \authorresponse{Thanks for pointing this out. We updated the description to make it clearer. We want to express that the proposed method is more stable than the baselines and ablations, which results in a smoother adaptation curve. With a more stable system identification procedure, we can simply use any iteration outputs to plug into the policy network instead of picking the ``best'' one from the adaptation iterations.}   
\end{enumerate}

\section*{References}
\begin{enumerate}[label=\textbf{\arabic*.}, leftmargin=1.5cm]
    \item Peide Huang, et al. ``What Went Wrong? Closing the Sim-to-Real Gap via Differentiable Causal Discovery'', 2023 Conference on Robot Learning, 2023.
\end{enumerate}

% Reviewer 3
\section*{Response to Reviewer 3}
Thanks for your comments. We are glad to hear that you found our paper is interesting and creative.  We made the corresponding improvement in the paper and addressed your concerns below.
\begin{enumerate}[label=\textbf{Q\arabic*.}, leftmargin=1.5cm]
    \item \reviewercomment{Justify the difference between using historical interaction data and current interaction data.}    
    
    \authorresponse{
    % Only using current iteration data would assume that the adaptation process following the Markov Decision Process (MDP), which is not always the case in the system identification.
    We compared our proposed approach, which leverages historical interaction data, with baseline methods that rely solely on current interaction data for environment parameter identification, such as Expert Distillation [1] and TuneNet [2]. Our results demonstrate significant performance improvements over these baselines in both tasks across sim-to-sim and sim-to-real transfer scenarios.}
    
    \item \reviewercomment{Reward function in reinforcement learning}    
    
    \authorresponse{For the table air hockey task, the reward function is defined as the inverse of the distance-to-goal. For the object scooping task, we used a sparse reward, which is 1 if the action selects the object center of mass, 0 otherwise.}

    \item \reviewercomment{Ablation on different iteration window $K$}    
    
      \authorresponse{We expanded our analysis to include the impact of different sequence lengths $K$ and transformer window sizes $k$ in the additional experiments section. The results of the ablation study on $K$ values are detailed and discussed in \hyperref[sec:exp_1]{Experiment 1}, while the ablations on the transformer window size ($k$, history length during inference) are presented in \hyperref[sec:exp_2]{Experiment 2}. Our findings indicate that the choice of $K$ has minimal impact on system identification performance, provided it falls within a reasonable range (e.g., between 7 and 9).}

    \item \reviewercomment{Figure 2 is not described in the text} 
    
    \authorresponse{We added the description for Figure 2 in Section III of the revised paper}
    
    \item \reviewercomment{For the experiment “Air Hockey Sim-to-Real Evaluation,” how were real-world trajectories measured.}   
    
    \authorresponse{As demonstrated in the supplementary videos on table air hockey sim-to-real performance, we had a top-down view of the air hockey table. In this setting, we equipped a camera on top of the air hockey table to track the puck trajectories. With the recorded trajectories, we can then compared with the simulation results through sum of L2 distance between real and simulation trajectories.}

    \item \reviewercomment{In Figure 6, when the adaptation iterations are too large, why do the normalized parameter differences of Right\_friction, Mallet\_damping, and Left\_damping increase?}  
    
    \authorresponse{We recall that the selected parameter transition sequence has a length \( K=7 \), and for training, we sample a subsequence of length \( k=4 \) from the entire sequence \( K \) to construct the dataset. Since the generated dataset ends at the 7th iteration, the model does not encounter any data points beyond this iteration during training. Additionally, the model has not seen any historical data sequences where all transitions exhibit optimal behavior during training. As a result, the adaptation steps beyond the 7th iteration involve unseen scenarios, classifying these steps as Out-of-Distribution (OOD) testing.
    Observing the results from the Capture + Linear Interpolation ablations, we see a sharp increase in parameter differences after iteration 7, likely due to the lack of exposure to well-performing sequences in the training data. In contrast, our proposed data generation approach enables Capture to generalize much better in OOD scenarios, as evidenced by the nearly flat or even decreasing trend in parameter difference plots across iterations. This behavior demonstrates that our framework is significantly more robust to OOD settings compared to baseline and ablation methods.
    }

    \item \reviewercomment{For the process of interacting with the environment, does the actual interactive environment need to be specially set?}    
    
    \authorresponse{No, we proposed a general framework for online SysID that does not need to specifically set any interactive environments. From our sim-to-sim evaluations, we randomly generated 100 pairs of sim and "real" environment parameters to comprehensively evaluate the model across 3 different seeds. For sim-to-real transfer, we also evaluated the object scooping model on three different daily objects with different center of mass positions, such as carrots, eggplants, and celery. In the table air hockey setting, we evaluated 15 trails with different fan voltages on both sides. We assume that such comprehensive evaluation in both simulation and the real-world can prove that our interactive environment does not need to be specifically set and can fit well in a general setting.}    
\end{enumerate}

\section*{References}
\begin{enumerate}[label=\textbf{\arabic*.}, leftmargin=1.5cm]
    \item Michael Laskin, et al. ``In-context Reinforcement Learning with Algorithm Distillation'', 2023 International Conference on Learning Representation, 2023.
    \item Adam Allevato, et al. ``TuneNet: One-Shot Residual Tuning for System Identification and Sim-to-Real Robot Task Transfer'', 2019 Conference on Robot Learning, 2019.
\end{enumerate}

% Reviewer 5
\section*{Response to Reviewer 5}
Thanks for your constructive and detailed comments. We made the corresponding improvements to the paper and addressed your concerns below.
\begin{enumerate}[label=\textbf{Q\arabic*.}, leftmargin=1.5cm]
    \item \reviewercomment{Justification on the monotonicity assumption.}    
    
    \authorresponse{Thanks for this interesting question. We modified the object scooping experiments to violate this monotonicity assumption, as detailed in \hyperref[sec:exp_4]{Experiment 4}. From Figure~\ref{fig:scoop_dist_env}, we observed that the lack of monotonicity indeed affects the task performance but still performs relatively well compared with the baseline methods. We added the monotonicity assumption in the reviser paper Section III.
    % \textcolor{red}{TODO: we will discuss this in the revised paepr}
    }
    
    \item \reviewercomment{Generalization to multi-task settings.}
    
    \authorresponse{In the real-world object scooping experiments, we successfully demonstrated the ability to scoop different objects using a single SysID model. Expanding this capability to a multi-task setting—such as enabling the model to perform both object scooping and table air hockey—is feasible within our proposed framework by incorporating a higher-dimensional environment parameter space and more generalized state representations. In this paper, our focus is on dynamics adaptation (environment parameter identification) for specific tasks that share the same state representation, action space, and environment parameter space. We sincerely appreciate the suggestion, as multi-task learning represents an exciting and promising direction for future exploration.}

    \item \reviewercomment{Model convergence and the stability of the learning process across different initial conditions.}    
    
    \authorresponse{The SysID causal transformer is trained with a supervised learning manner, where we collected 80000 adaptation iteration sequences using randomized binary search algorithms. We assume that the supervised learning algorithms generally do not get affected too much by initial conditions. Still, we plotted some training curves of our SysID causal transformer in the additional experiment section for your clarifications in \hyperref[sec:exp_6]{Experiment 6}.}

    \item \reviewercomment{Comparison with recent baselines such as COMPASS[1]}    
    
    \authorresponse{We added the COMPASS baseline in the \hyperref[sec:exp_3]{Experiment 3}. We observed that COMPASS was not able to perform as well as CAPTURE in both the table air hockey and object scooping settings after comprehensive sim-to-sim evaluations.}

    \item \reviewercomment{The robustness of the CAPTURE model to noise in real-world data, such as sensor noise or pose disturbances, is not explicitly addressed.}    
    
    \authorresponse{In the original draft, we used a top-down camera to capture the puck trajectories in the table air hockey task and compared them with the simulated trajectories. With this camera, we inevitably have the noise from camera data. In the object scooping task, to mitigate the effect of noisy point cloud data, we used a classifier that labels the object's tilting direction instead of requiring the tilting angle of the object. In this revision, we added robustness evaluations on both tasks in the sim-to-sim setting with added pose disturbance and trajectory noises as shown in \hyperref[sec:exp_7]{Experiment 7}. The results show that the noisy state inputs do not significantly degrade the parameter estimation performance, given the existence of historical data.}

    \item \reviewercomment{As shown in some figures and tables in the manuscript, it seems that CAPTURE tends to show an interesting 'overfit' manner after iterations. Is there any further analysis on this?}    
    
    \authorresponse{We recall that the selected parameter transition sequence has a length \( K=7 \), and for training, we sample a subsequence of length \( k=4 \) from the entire sequence \( K \) to construct the dataset. Since the generated dataset ends at the 7th iteration, the model does not encounter any data points beyond this iteration during training. Additionally, the model has not seen any historical data sequences where all transitions exhibit optimal behavior during training. As a result, the adaptation steps beyond the 7th iteration involve unseen scenarios, classifying these steps as Out-of-Distribution (OOD) testing.
    Observing the results from the Capture + Linear Interpolation ablations, we see a sharp increase in parameter differences after iteration 7, likely due to the lack of exposure to well-performing sequences in the training data. In contrast, our proposed data generation approach enables Capture to generalize much better in OOD scenarios, as evidenced by the nearly flat or even decreasing trend in parameter difference plots across iterations. This behavior demonstrates that our framework is significantly more robust to OOD settings compared to baseline and ablation methods.}

    \item \reviewercomment{Justification on Linear Interpolation and random shuffling.}   
    
    \authorresponse{We implemented a ``randomized" linear interpolation approach by randomly selecting $K$ points between the source and target. These points are then ordered from closest to the source to closest to the target to generate adaptation sequences for the training set. In terms of adding more randomization, such as shuffling those orders of randomly sampled numbers, we found it less intuitive than our approach. The goal of generating parameter transition sequences is to obtain a process that can get gradually better, where if we randomly shuffle the order, the generated sequence would not retain such properties. Eventually, the SysID causal transformer might learn a random prediction from this shuffled dataset.}

    \item \reviewercomment{Some failure cases and method limitations may better help readers understand the method and its performance.}  
    
    \authorresponse{We added the limitations of our current experiments in the updated version. One interesting sub-optimal behavior that we noticed is that the model did not perform optimally compared with humans in the real-world eggplant scooping task. Humans, as a near-optimal dynamics adaptation algorithm, know that as long as I successfully lift the object, I do not need to explore other space. However, with CAPTURE, it still explored the environment a bit before coming back to the center of mass position. Another interesting future work is to extend the proposed frameworks to multi-tasking learning, given that we only focus on adaptation of single-task dynamics in this paper. With more generalizable state representations and action space, it would better fit our model to multi-task settings. }    
\end{enumerate}


% Additional Material
\clearpage
\section*{Additional Experiments}

\subsection*{Experiment 1: Ablation on different parameter transition sequence $K$ during data generation.}
\label{sec:exp_1}
    
    As suggested by reviewers, running more ablation on the parameter transition sequence $K$ would justify the chosen hyper-parameters in our setting. We varied the generated sequence length $K$, ranging from 5 to 13, as shown in Figure~\ref{fig:different_K_push_one}.
    We collected 100 pairs of sim and simulated real environment parameters to comprehensively evaluate the performance under different initial conditions.
    We can observe that different $K$ values do not steer too much on the performances, where only some samples have inferior behaviors compared to others, such as when $K = 5$ and $K = 13$. Overall, we can observe that the varied length of transition sequences does not affect the performance significantly if chosen within a reasonable range between 7 and 9. Since the proposed randomized binary search algorithm is independent of the dimensions of state trajectories, action space, and environment parameter spaces, this range theoretically should fit well into other settings as well.
    \begin{figure}[h]
        \centering
        \includegraphics[width=\linewidth]{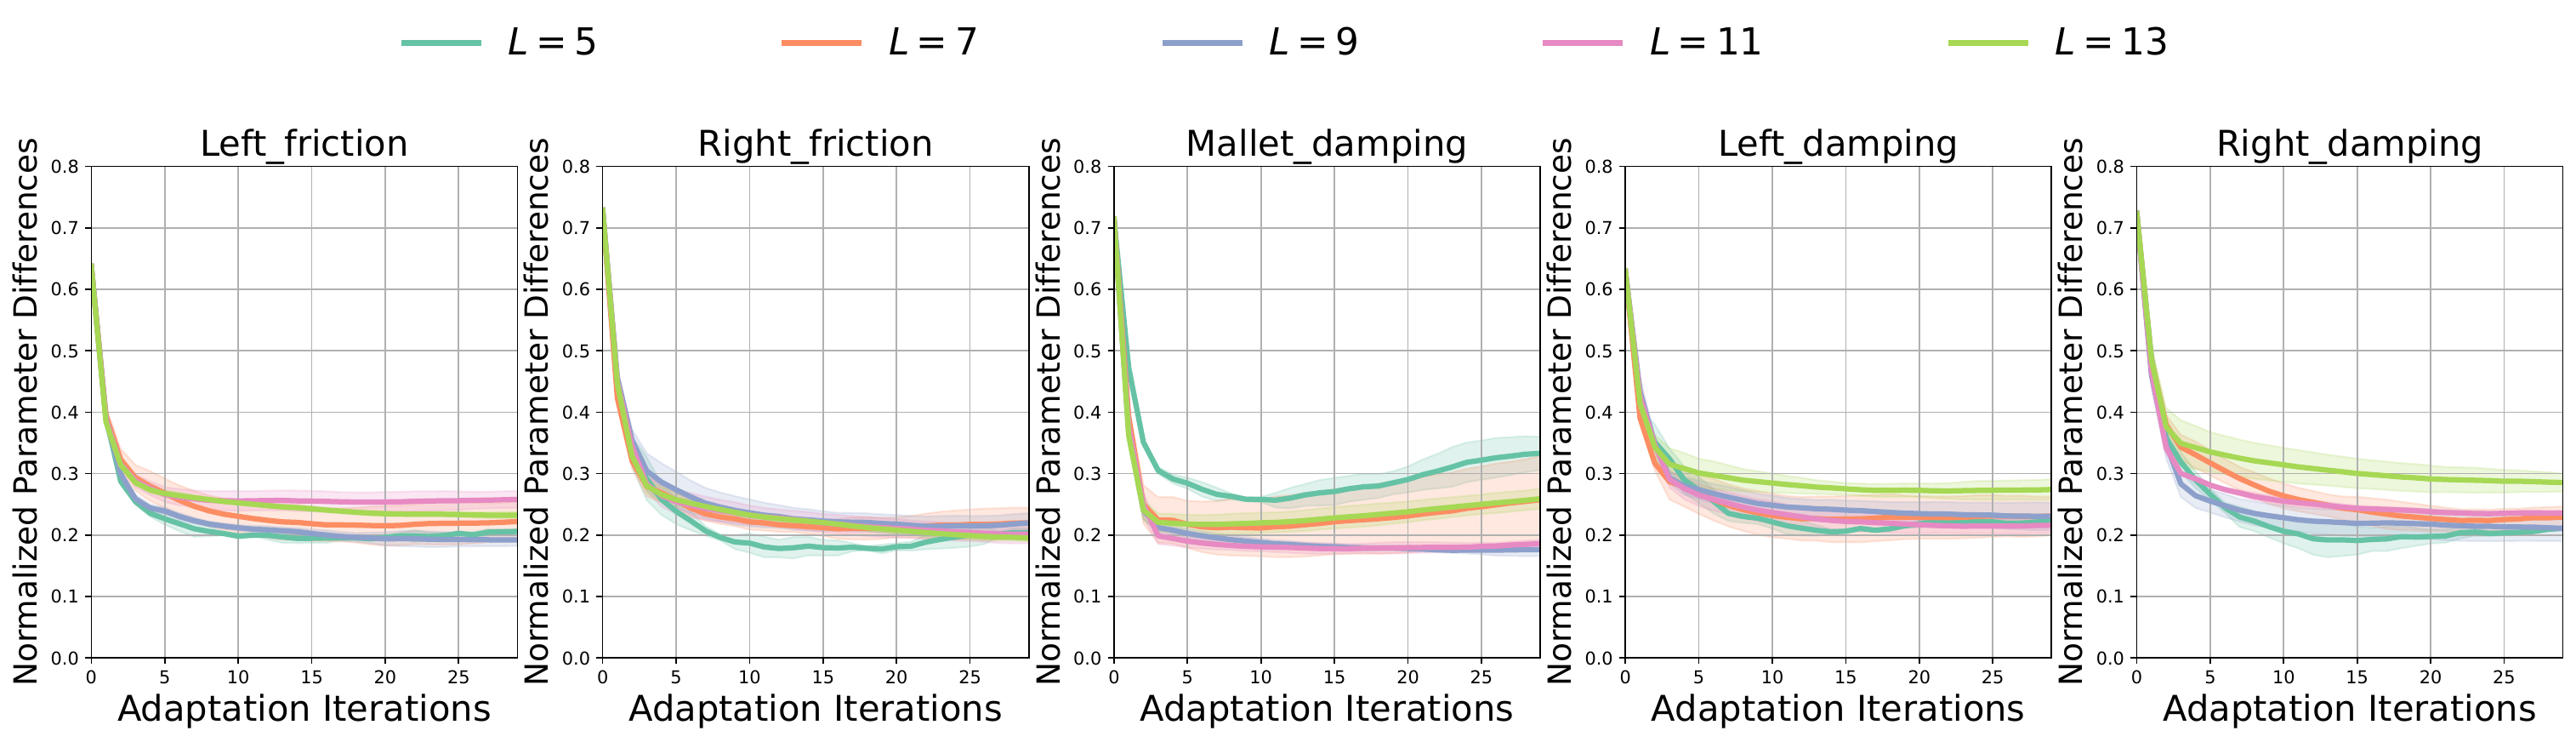}
        \caption{Table air hockey sim-to-sim transfer SysID performance across different parameter transition sequence length $K$. }
        \label{fig:different_K_push_one}
    \end{figure}

    % \begin{figure}[h]
    %     \centering
    %     \includegraphics[width=0.5\linewidth]{hisotry_push_one_traj.pdf}
    %     \caption{Table air hockey sim-to-sim transfer SysID average trajectory differences across different parameter transition sequence length K. }
    %     \label{fig:different_K_push_one_traj}
    % \end{figure}


    By observing the object scooping behavior shown in Figure~\ref{fig:different_K_scoop}, we found a similar pattern with the table air hockey task on parameter estimation performances.
    \begin{figure}[h]
        \centering
        \includegraphics[width=0.7\linewidth]{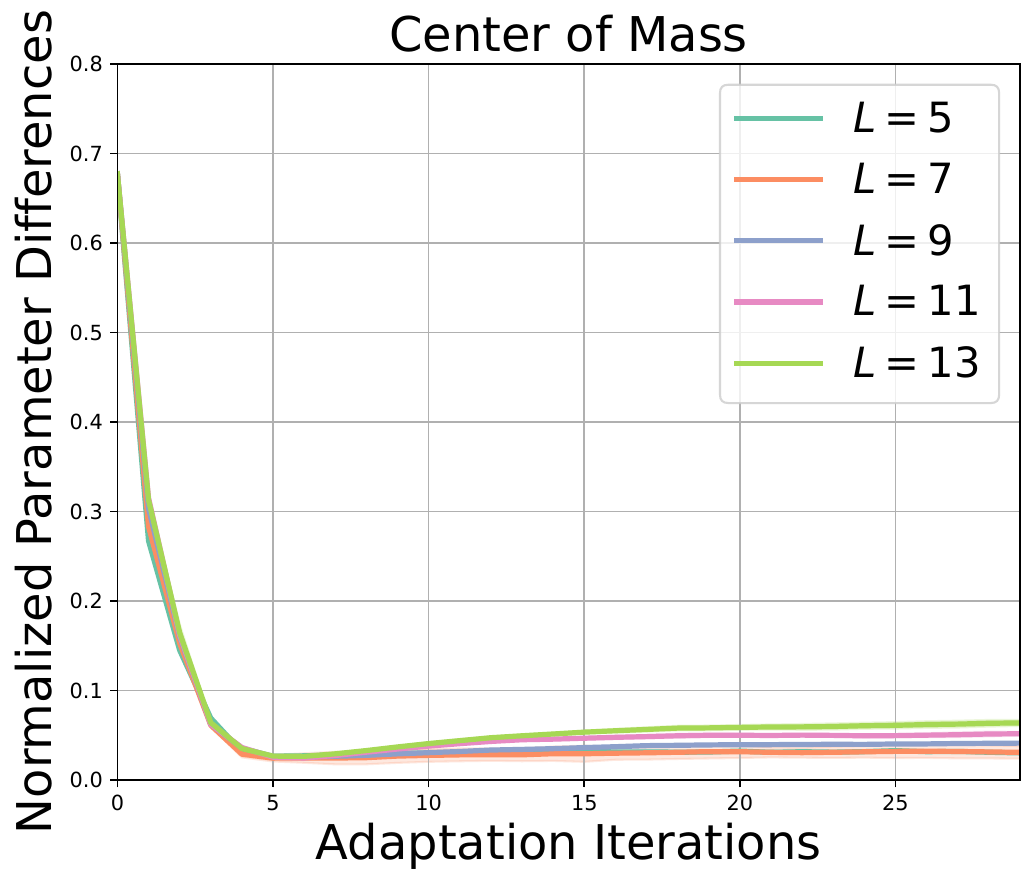}
        \caption{Object Scooping sim-to-sim transfer SysID performance across different parameter transition sequence length $K$. }
        \label{fig:different_K_scoop}
    \end{figure}

    
\clearpage
\subsection*{Experiment 2: Ablation on different window size $k$.}
\label{sec:exp_2}
    
    As suggested by reviewers, we added more ablations on different window size $k$ of the transformer models. We collected 100 pairs of sim and simulated real environment parameters to fully assess performance under different initial conditions. To evaluate the performance dependency on the length of the window size $k$, we kept the generated transition sequence length $K = 7$ and varied the window size $k$ from 2 to 6, as shown in Figure~\ref{fig:different_k_push} and Figure~\ref{fig:different_k_scoop}. We can observe that ($k = 2$) and ($k = 3$) perform better on most of the environment parameters, whereas the longer window size tends to perform worse, especially in later iterations. This is a reasonable behavior because larger window sizes are easier to overfit to the training data sequence (in this case, $K=7$) and lead to worse performance on Out-of-Distribution(OOD) generalization after adaptation iteration exceeds $K$. Conversely, a smaller window size learns from a sampled subsequence from the whole generated transition sequences, which focuses on local features rather than long-horizon features. Such structure would enhance the generalizability to OOD settings. Conclusively, the value of window size depends on the state trajectory complexity of the dynamical systems. If the environment requires more steps to explore the environments, it would generally need more history(window size) to predict the next-step environment parameters and vice versa. 
    
    \begin{figure}[h]
        \centering
        \includegraphics[width=\linewidth]{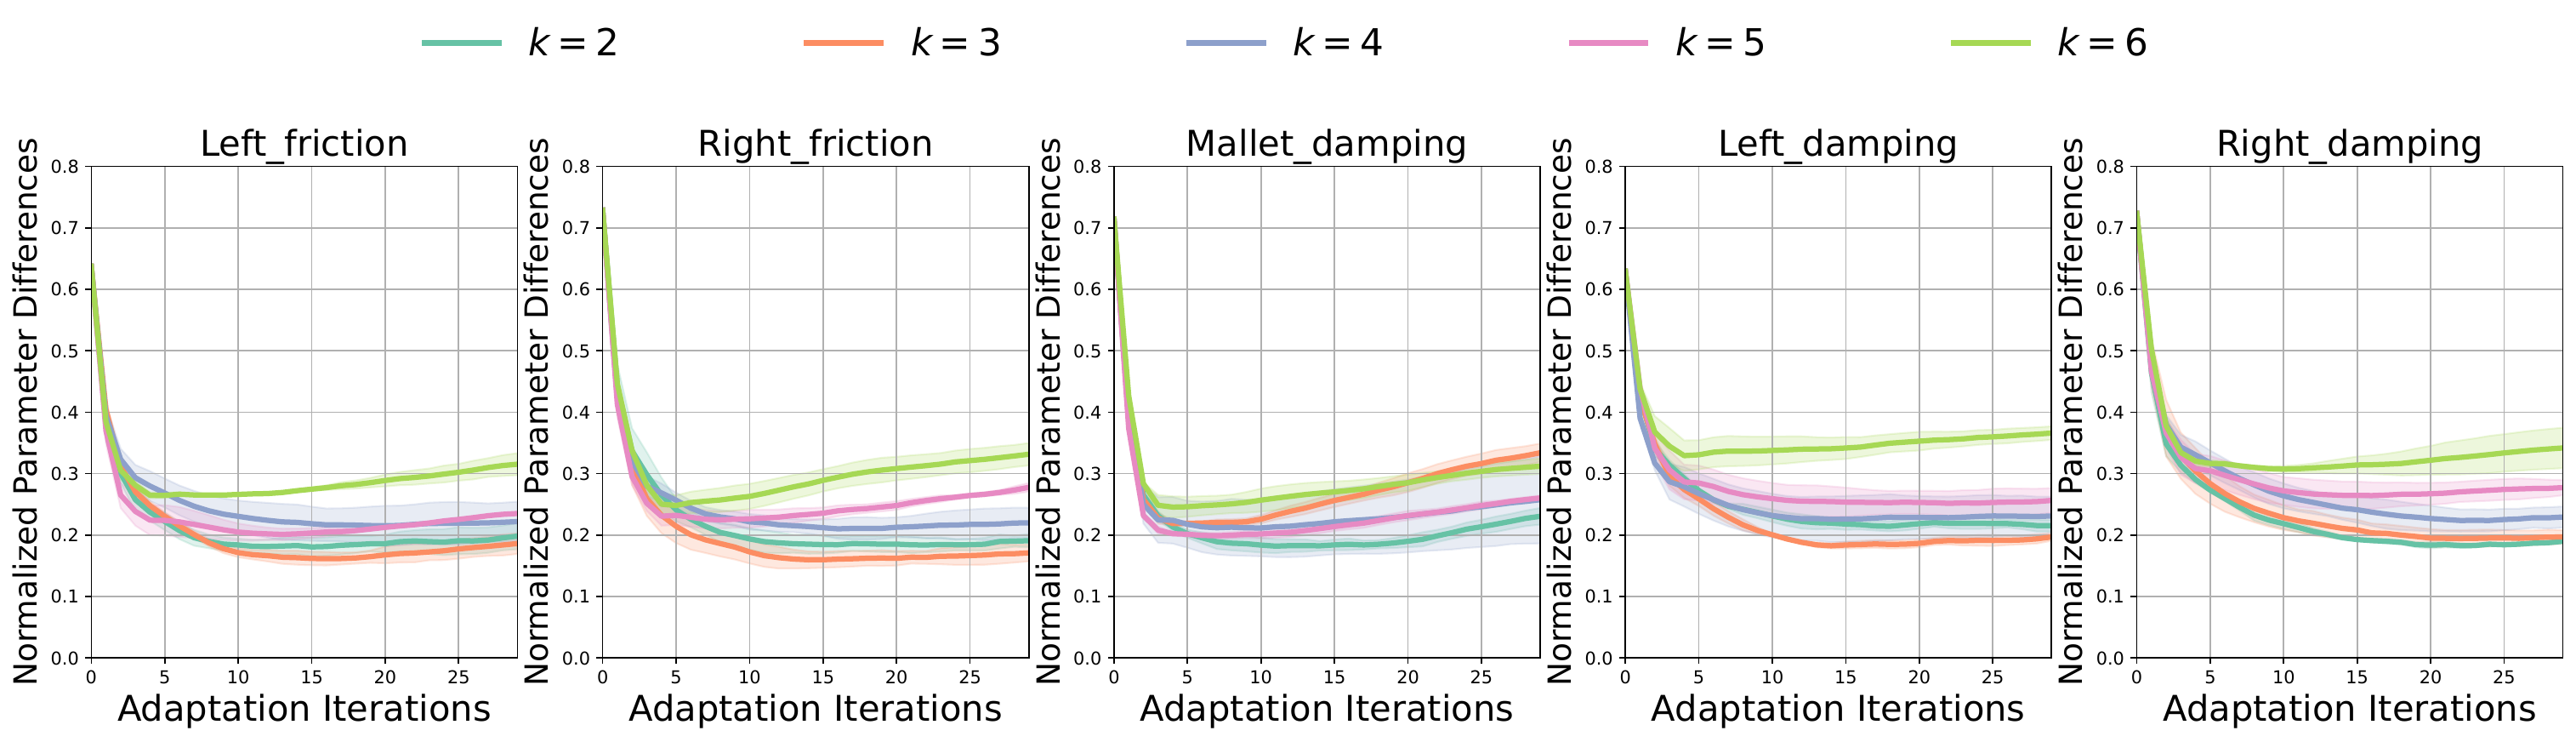}
        \caption{Table air hockey sim-to-sim transfer SysID performance across different window sizes. }
        \label{fig:different_k_push}
    \end{figure}
    
    \begin{figure}[h]
        \centering
        \includegraphics[width=0.7\linewidth]{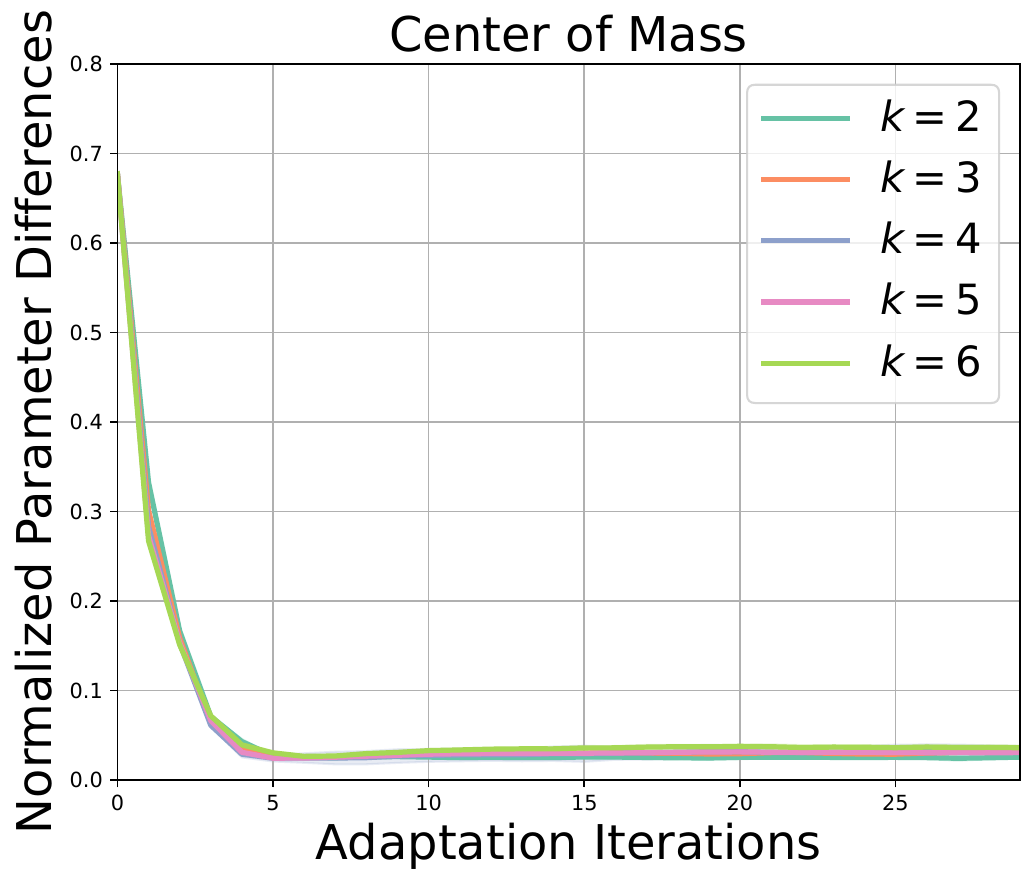}
        \caption{Object Scooping sim-to-sim transfer SysID performance across different window sizes. }
        \label{fig:different_k_scoop}
    \end{figure}


\clearpage
\subsection*{Experiment 3: Added recent SysID baselines (COMPASS)}
\label{sec:exp_3}
    
    As suggested by multiple reviewers, by adding COMPASS as our additional baseline method, we tried to align with the paper setting as closely as possible. In the original paper, the authors proposed to collect 10 trajectories to estimate the environment parameters. With the CAPTURE setting, since we only need to collect one trajectory at every iteration, we will compare the results with COMPASS through 10 iteration adaptation sequences. Moreover, since we only provided the ``useful" environment parameters to CAPTURE, we also set the COMPASS causal graph as full\_graph to ensure that all environment parameters will be optimized. We evaluated COMPASS with 50 random source and target environment parameters across 3 different seeds. The results for both experiments are shown in Figure~\ref{fig:push_one_compass} and Figure~\ref{fig:scoop_compass}. We can observe that COMPASS had a good trend of aligning the center of mass in the object scooping tasks but converging comparatively slower. In the table air hockey setting, COMPASS was not able to perform well in this setting even though some of the environment parameters have good starting points (left\_friction). 
        \begin{figure}[h]
        \centering
        \includegraphics[width=\linewidth]{push_one_combined_context_history.pdf}
        \caption{Table air hockey sim-to-sim transfer with added baseline. }
        \label{fig:push_one_compass}
    \end{figure}
        \begin{figure}[h]
        \centering
        \includegraphics[width=0.7\linewidth]{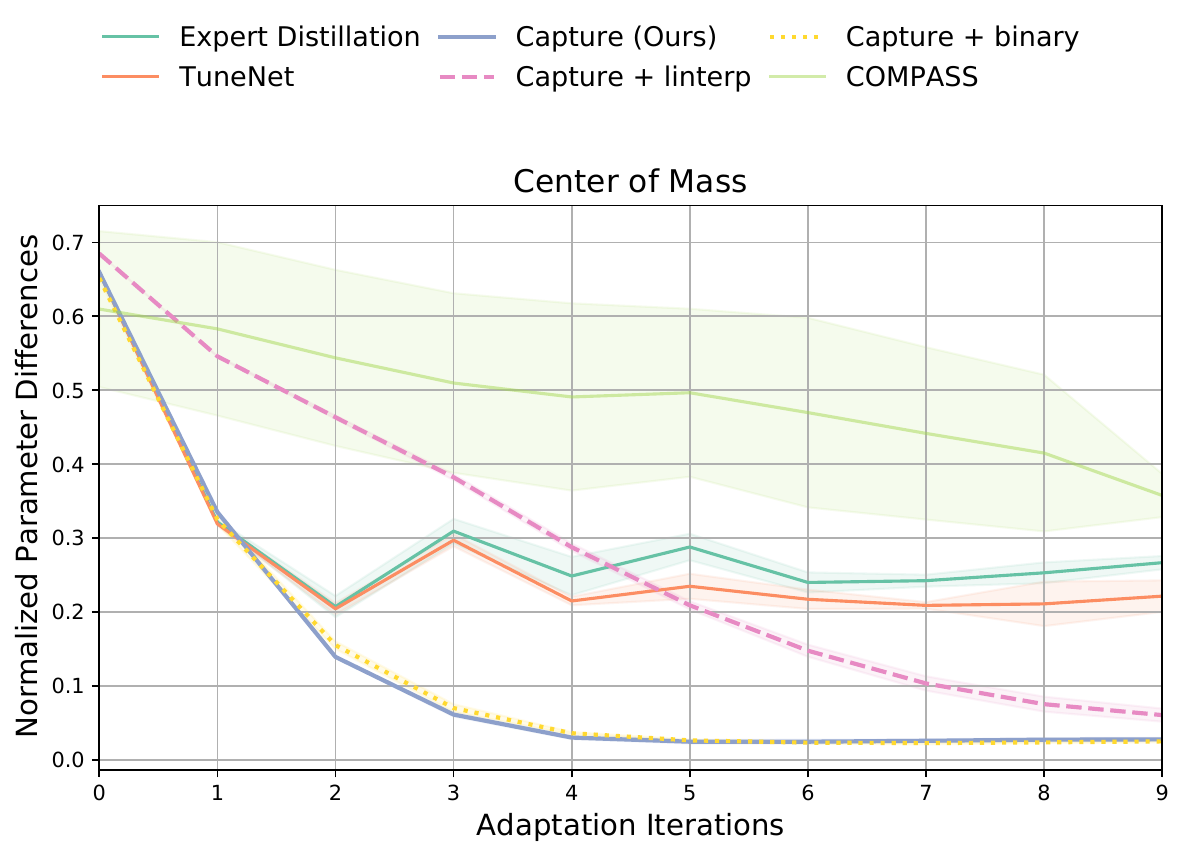}
        \caption{Object Scooping sim-to-sim transfer with added baseline.}
        \label{fig:scoop_compass}
    \end{figure}

    \clearpage
    
    % Let $\tau = f(\epsilon)$ where $\tau$ is the state trajectories, $f$ is the simulator, and $\epsilon$ is the environment parameters. Our goal is to identify the environment parameter $\tau^{real}$
    
\subsection*{Experiment 4: CAPTURE performance within a non-monotonic relationship between environment parameters and state trajectories.}
\label{sec:exp_4}
Indeed, the binary search method relies on the monotonic relationship between environment parameters and state trajectories under the same action. We also observed that most physical properties defined in simulators inherently follow such monotonic relationships. For example, in our experiments, parameters like friction and damping consistently influence the behavior of state trajectories in predictable ways. Increasing the damping coefficient typically results in slower system responses, while higher friction values lead to reduced sliding distances. 

While this assumption holds true for many environment parameters, we acknowledge that there may be cases where the relationship between parameters and state trajectories is non-monotonic. Without such an assumption, the binary search process would lack the framework to accurately update these bounds.However, state trajectories are not strictly required when generating transition sequences for the environment parameter identification process, as the ground truth of the environment parameters is accessible. As a result, it is possible to generate reasonable transition sequences even in the presence of a non-monotonic relationship between environment parameters and state trajectories. 

To validate this assumption, we modified the observation of the scoop environment to represent the distance between the scoop point and the center of mass. The relationship between the state and the environment parameter under the same action is illustrated in Figure~ \ref{fig:scoop_dist_env}. This figure highlights that the relationship between the observation and the center of mass is non-monotonic, confirming the validity of our approach.


    \begin{figure}[h]
        \centering
        \includegraphics[width=1.0\linewidth]{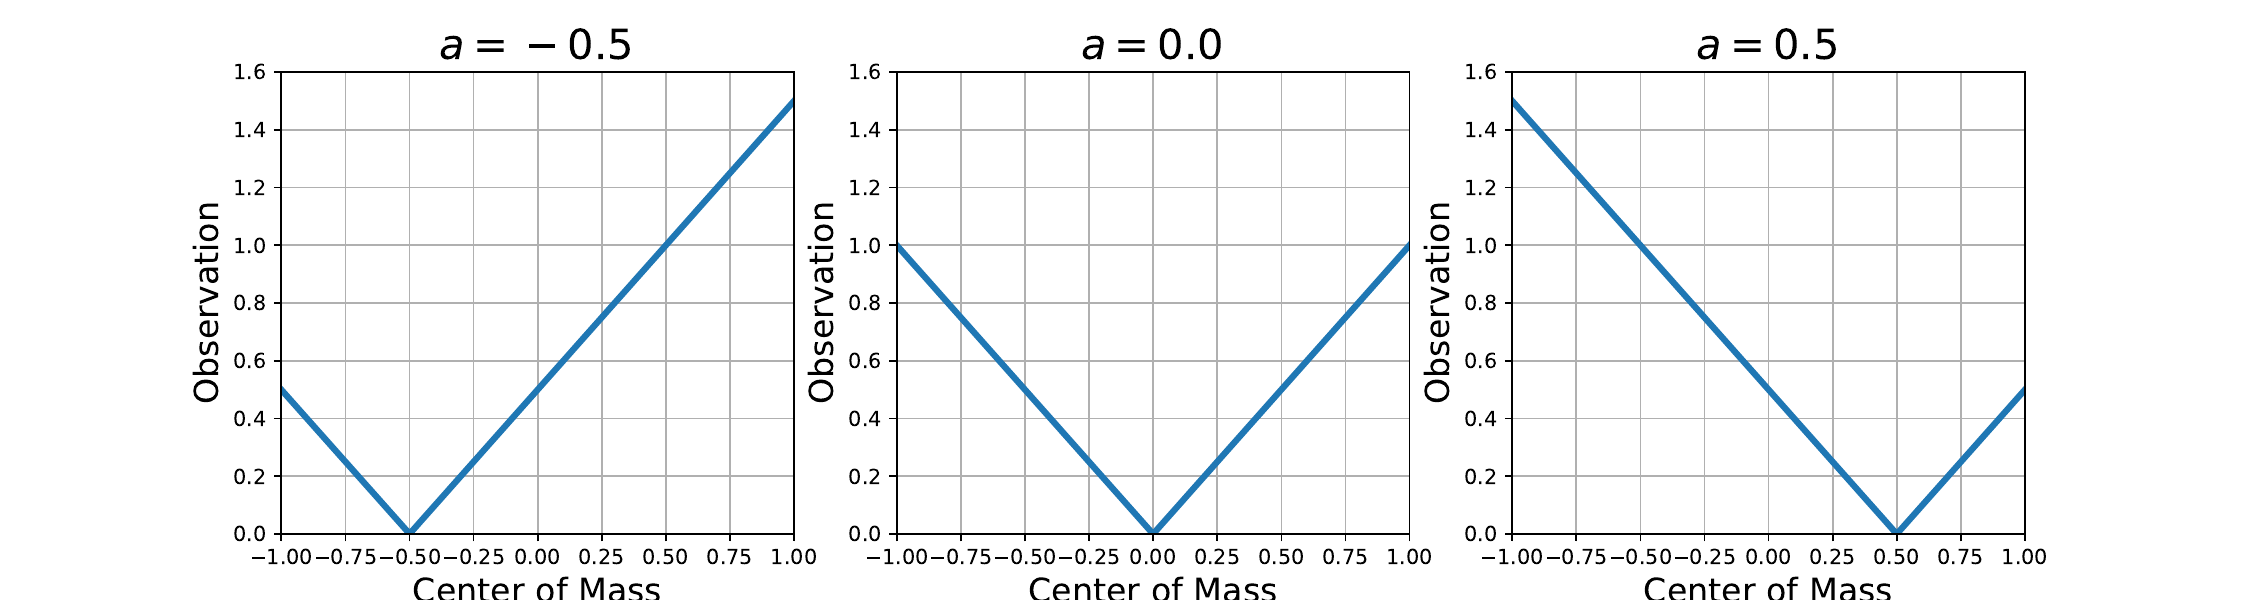}
        \caption{Relationship between the observation and environment parameter under same actions for the non-monotonic scoop environment}
        \label{fig:scoop_dist_env}
    \end{figure}

    We evaluated our method, CAPTURE, against two baseline methods, Expert Distillation and TuneNet, in this environment. We collected 100 pairs of sim and simulated real environment parameters to fully assess performance under different initial conditions. The results are presented in Figure~\ref{fig:original_scoop_dist}.

    \begin{figure}[h]
        \centering
        \includegraphics[width=0.47\linewidth]{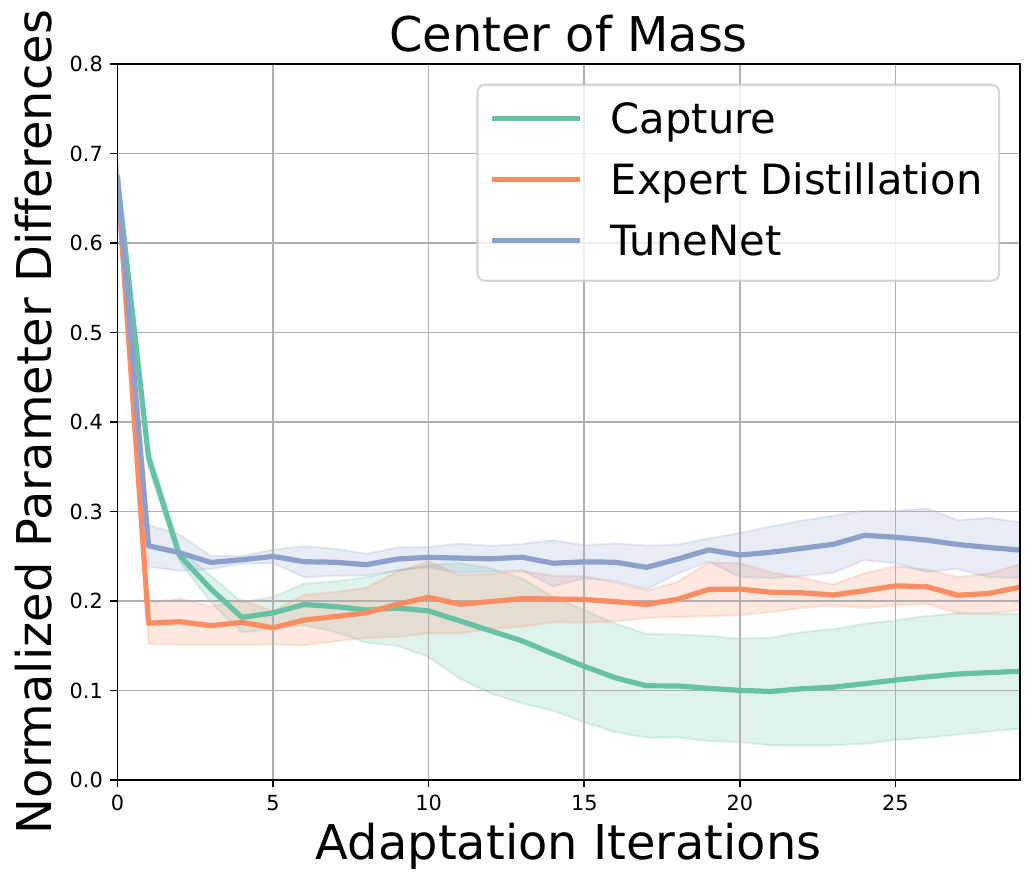}
        \caption{Performance of CAPTURE, Expert Distillation, TuneNet for non-monotonic scoop environment.}
        \label{fig:original_scoop_dist}
    \end{figure}

    Our observations indicate that CAPTURE struggles to identify the correct environment parameter during the first few iterations. However, after the 10th iteration, the error gradually decreases, and CAPTURE still outperforms the baseline methods. 
    Therefore, even in environments with no monotonic relationship between state trajectories and environment parameters, CAPTURE maintains superior performance compared to the baseline approaches.

    \clearpage
\subsection*{Experiment 5: Balance between exploration and exploitation.}
\label{sec:exp_5}

    The binary search method used in CAPTURE is a deterministic algorithm that narrows the bound of dynamic parameters for each interaction. Therefore, there is no hyperparameter to balance between exploration and exploitation. 
    However, to investigate the impact of the exploration-exploitation trade-off on the performance of our method, we introduced a new hyperparameter, $\Gamma$, which adjusts the ratio between exploration and exploitation. 
    Algorithm~\ref{alg:data_collection} illustrates the implementation, with modifications highlighted in red for clarity.

    \begin{algorithm}[h]
    \caption{Source-to-Target SysID Iteration Generation with Additional Exploration}
    \label{alg:data_collection}
    \begin{algorithmic}[1]
        \State Initialize data buffer $\mathcal{D}$
        \State Choose parameter transition iteration length $K$
        \State Choose symmetric beta distribution parameter ${\alpha}$
        \State \textcolor{red}{Choose exploration parameter $\gamma \in [0, 1)$}
        \For{$n = 1$ to $N$}  \Comment{This loop can be run in parallel}
            \State Sample $\epsilon^{\text{source}}, \epsilon^{\text{target}}$ from space $\mathcal{E}$
            \State Let $l$ be the dynamic lower bound of space $\mathcal{E}$
            \State Let $u$ be the dynamic upper bound of space $\mathcal{E}$
            \State Set $\epsilon_0 = \epsilon^{\text{source}}$
            \For{$i = 0$ to $K$}
                \State Sample action $a_i \sim \pi(a_{i} \mid s_0, \epsilon_{i})$
                \State $\tau^{\text{source}}_{i} \leftarrow$ rollout in $sim(\epsilon_{i})$ with $a_i$
                \State $\tau^{\text{target}}_{i} \leftarrow$ rollout in $sim(\epsilon^{\text{target}})$ with $a_i$
                \For{$j = 1$ to $\dim(\mathcal{E})$}
                    \State \textcolor{red}{Sample $\gamma \sim \text{Uniform}[0, 1]$}
                    \If{\textcolor{red}{$\gamma > \Gamma ^ {i}$}}
                        \If{$\epsilon_i[j] < \epsilon^{\text{target}}[j]$}
                            \State Update lower bound: $l[j] = \epsilon_i[j]$
                        \Else
                            \State Update upper bound: $u[j] = \epsilon_i[j]$
                        \EndIf
                    \EndIf
                    \State Sample $r$ from $\mathrm {B}(\alpha, \alpha)$ 
                    \State Set $\epsilon_{i+1}[j] = r \left(u[j] - l[j]\right) + l[j]$
                \EndFor 
                \State Store trajectory $h[i] = \{\epsilon_{i}, a_{i}, \tau^{\text{source}}_i, \tau^{\text{target}}_i\}$
            \EndFor 
            \State Update data buffer: $\mathcal{D} \leftarrow \mathcal{D} \cup h$
        \EndFor 
    \end{algorithmic}
\end{algorithm}

As illustrated in Algorithm~\ref{alg:data_collection}, the modified method updates the upper and lower parameter bounds only when the sampled $\gamma > \Gamma^i$ at the $i$-th step of a transition sequence. Consequently, a larger $\Gamma$ value permits the transition sequence to engage in more extensive exploration during the initial stages. In contrast, a smaller $\Gamma$ value rapidly narrows the gap between the upper and lower bounds, causing the sequence to allocate a greater proportion of its focus to exploitation.

For subsequent experiments, we set $\Gamma = 0.5$ and evaluate its sim-to-sim performance in both table air hockey and object scooping environments, each with 3 random seed across 100 different pairs of simulation and simulated real environment parameters. We designate this approach as ``Capture + explore", as our original method can be considered a special case with $\Gamma = 0$, thereby foregoing additional exploration. 

As shown in Figure~\ref{fig:explore_scoop}, ``Capture + explore" slightly decreased performance compared to the original method; however, this difference is negligible.

Figures~\ref{fig:explore_push_one_context} demonstrate that ``Capture + exploration" improves overall performance by learning from transition sequences with additional exploration. This improvement is expected because, in the table air hockey experiment, the plate only moves to either the left or right side, necessitating more exploration to achieve a more accurate estimation.

In conclusion, adjusting the level of exploration can be beneficial and positively impact the results; however, whether additional exploration is required largely depends on the specific environment. 
% Future work will explore adaptive exploration strategies tailored to diverse environmental conditions to further enhance performance.

\begin{figure}[h]
    \centering
    \includegraphics[width=0.6\linewidth]{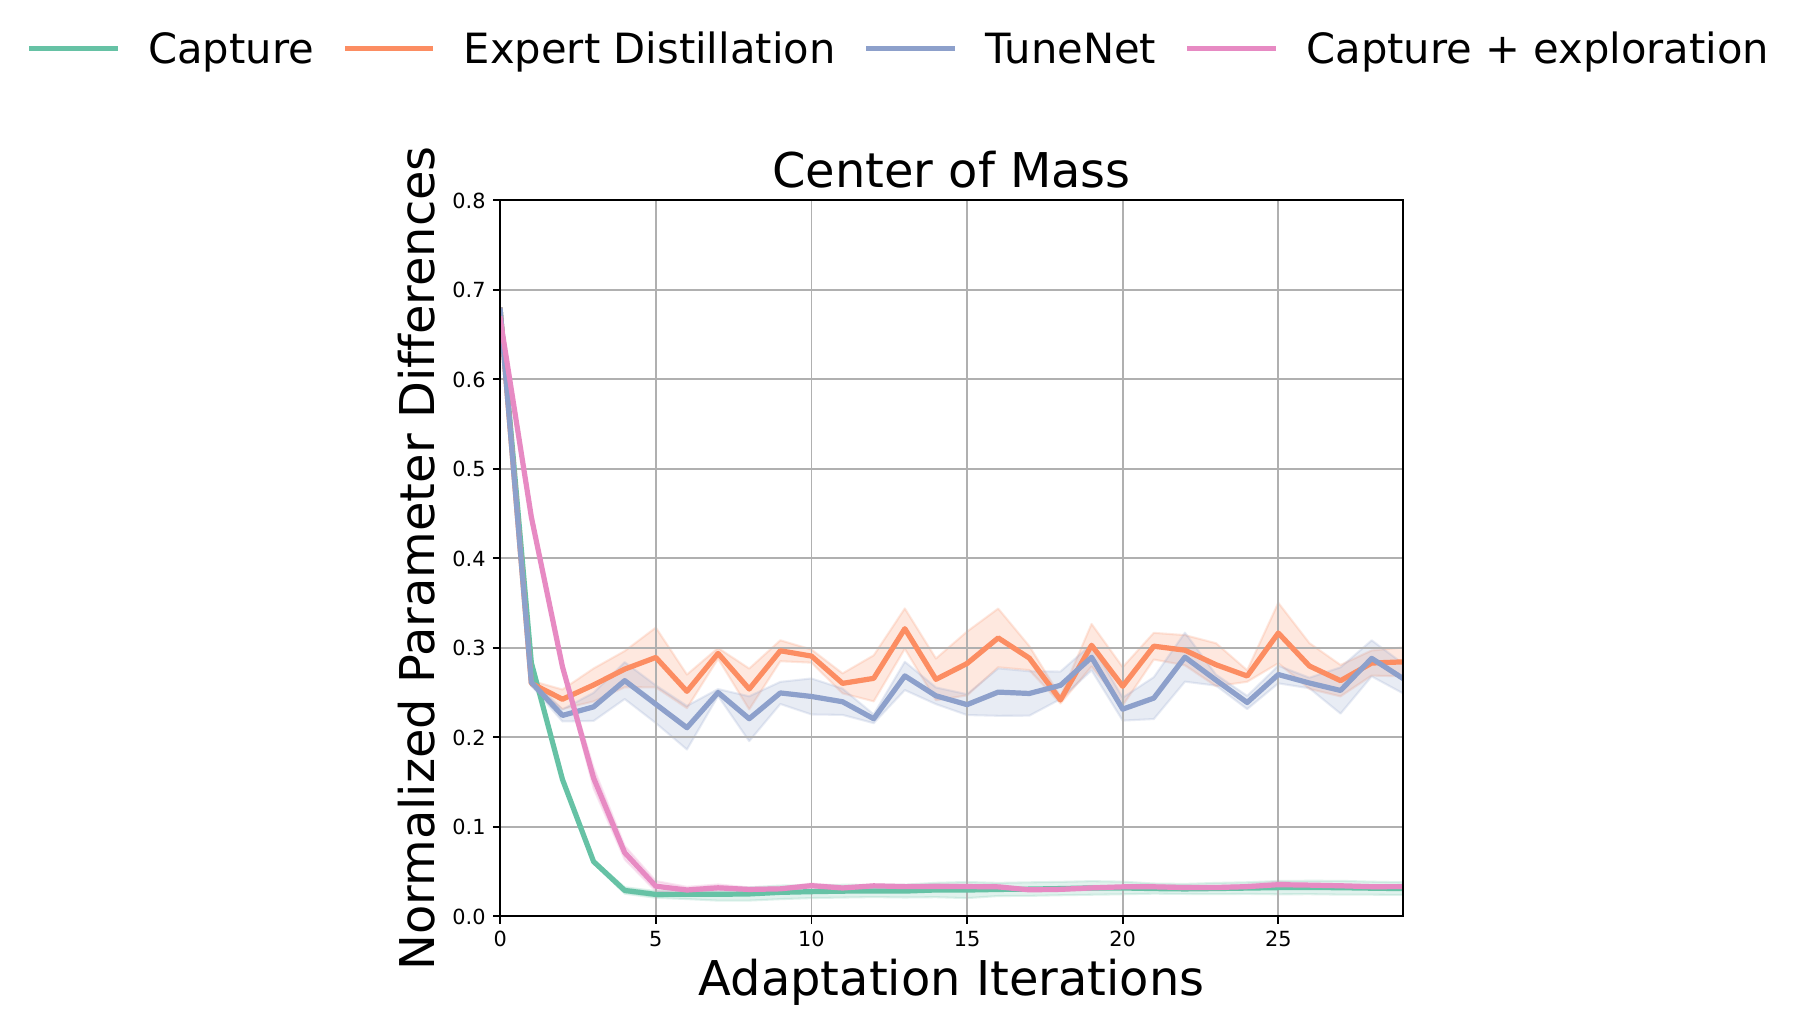}
    \caption{Object scooping sim-to-sim transfer SysID performance. ``Capture + explore" achieves performance comparable to the original implementation, although it requires more iterations due to exploration.}
    \label{fig:explore_scoop}
\end{figure}

\begin{figure}[h]
    \centering
    \includegraphics[width=\linewidth]{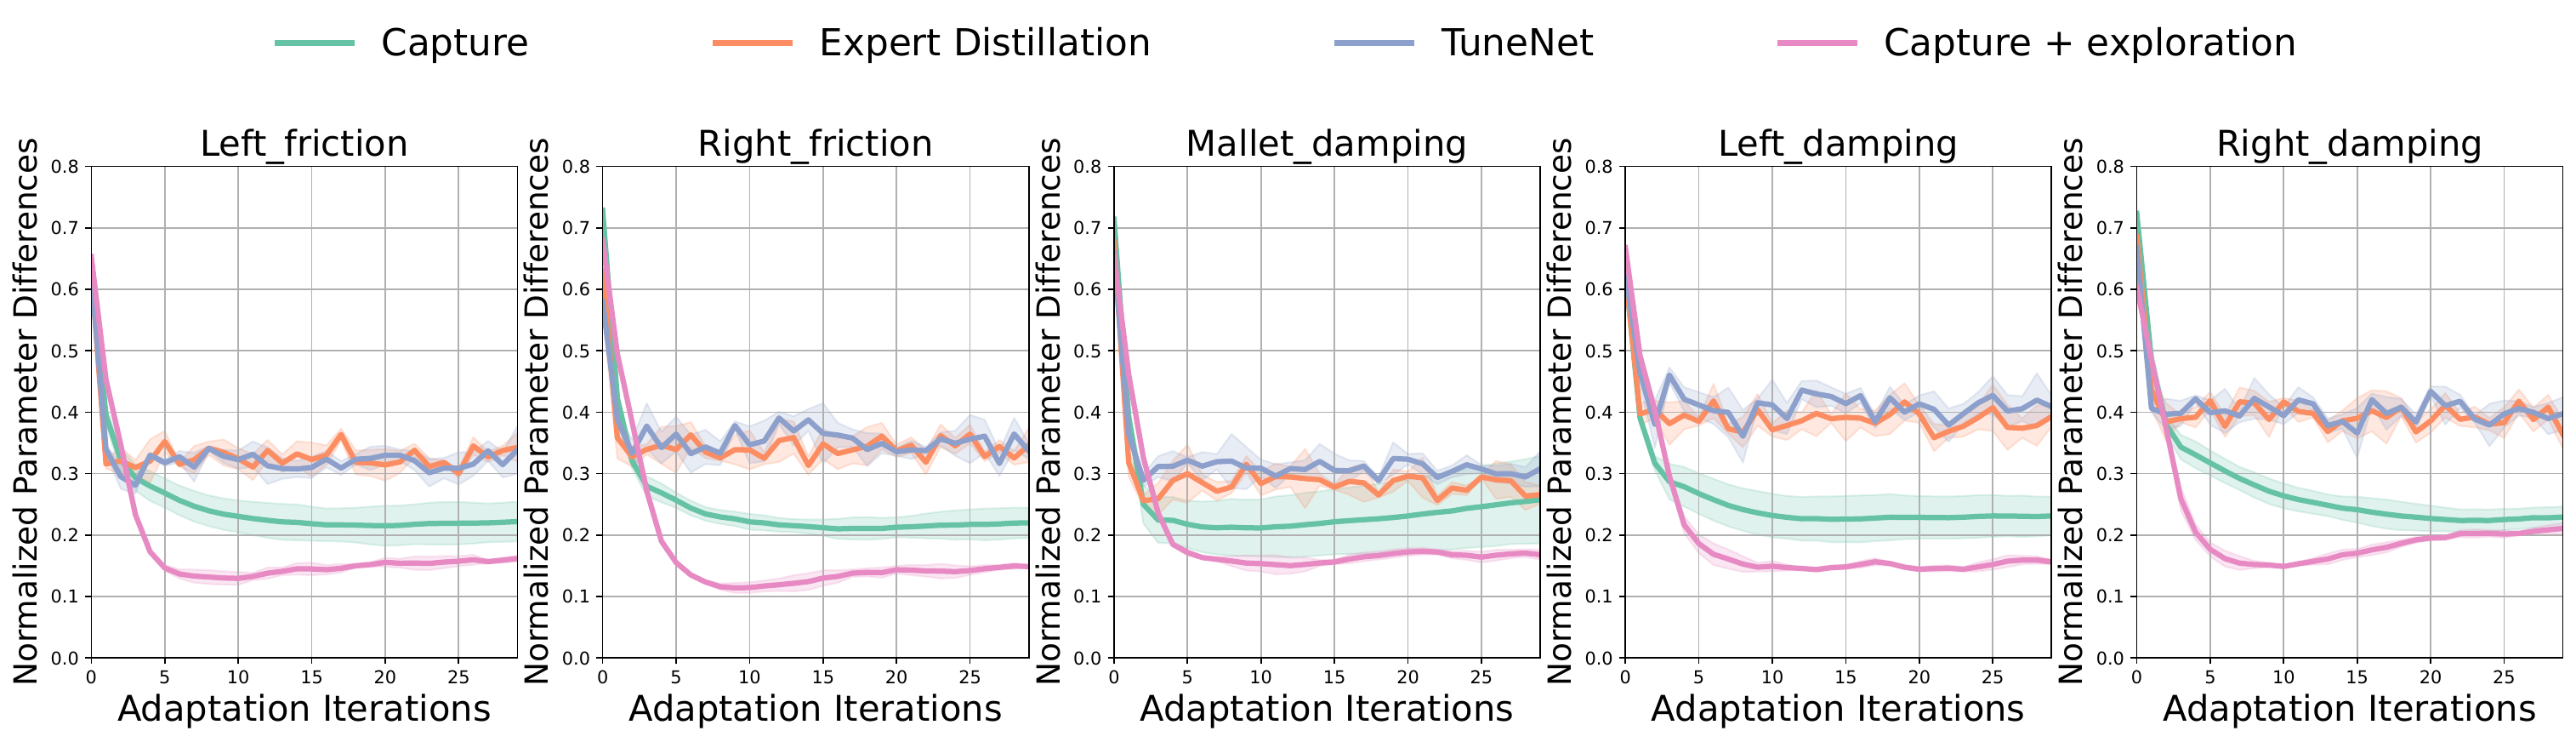}
    \caption{Table air hockey sim-to-sim transfer SysID performance. ``Capture + explore" consistently achieves the fastest and most significant reduction in differences, outperforming other methods. It also shows lower variance suggesting more consistent performance.}
    \label{fig:explore_push_one_context}
\end{figure}

% \begin{figure}[h]
%     \centering
%     \includegraphics[width=\linewidth]{explore_push_one_traj.pdf}
%     \caption{Table air hockey sim-to-sim transfer SysID trajectory difference. ``Capture + explore" achieves the lowest trajectory differences throughout the adaptation process, demonstrating its superior performance in learning accurate trajectories quickly.}
%     \label{fig:explore_push_one_traj}
% \end{figure}






    

    % Like other physical simulators, Mujoco has a lot of environment parameters that can be adjusted, including friction coefficient, damping ratio, stiffness, 

    


\clearpage
\subsection*{Experiment 6: Discuss computation data, time, and convergence plots}
\label{sec:exp_6}

    
    To further address the reviewers' concern on the computation overhead and the training curves, we added more plots on our training curves and corresponding responses in this ection.
    \begin{itemize}
        \item \textbf{Discussion on the computation overhead:} It is true that CAPTURE requires more training time compared to baseline methods. The additional computation time primarily arises from the need to learn longer sequences, whereas baseline methods only require learning a one-step matching policy. However, we assume that generating training data in simulation is computationally inexpensive, and we prioritize task performance over model training time. 

        The model structure of the baseline methods inherently limits their performance, regardless of the amount of training data or time provided. Furthermore, during the real-world adaptation process, where trajectory collection is costly, CAPTURE requires only one trajectory per adaptation iteration. This approach remains practical in most scenarios and balances efficiency with performance effectively.

        \item  \textbf{Discussion on the training plots:} As shown in Figure~\ref{fig:traing_loss}, we present the training curve of the transformer model across three seeds along with the corresponding evaluation results at each training step. For the evaluation during training, we report the results after the 7th adaptation iteration. Notably, the training losses across different seeds show minimal variation, indicating consistent training performance. The variance observed in the training evaluations is primarily attributed to the variability in the task policy.

        \begin{figure}[h]
            \centering
            \includegraphics[width=0.8\linewidth]{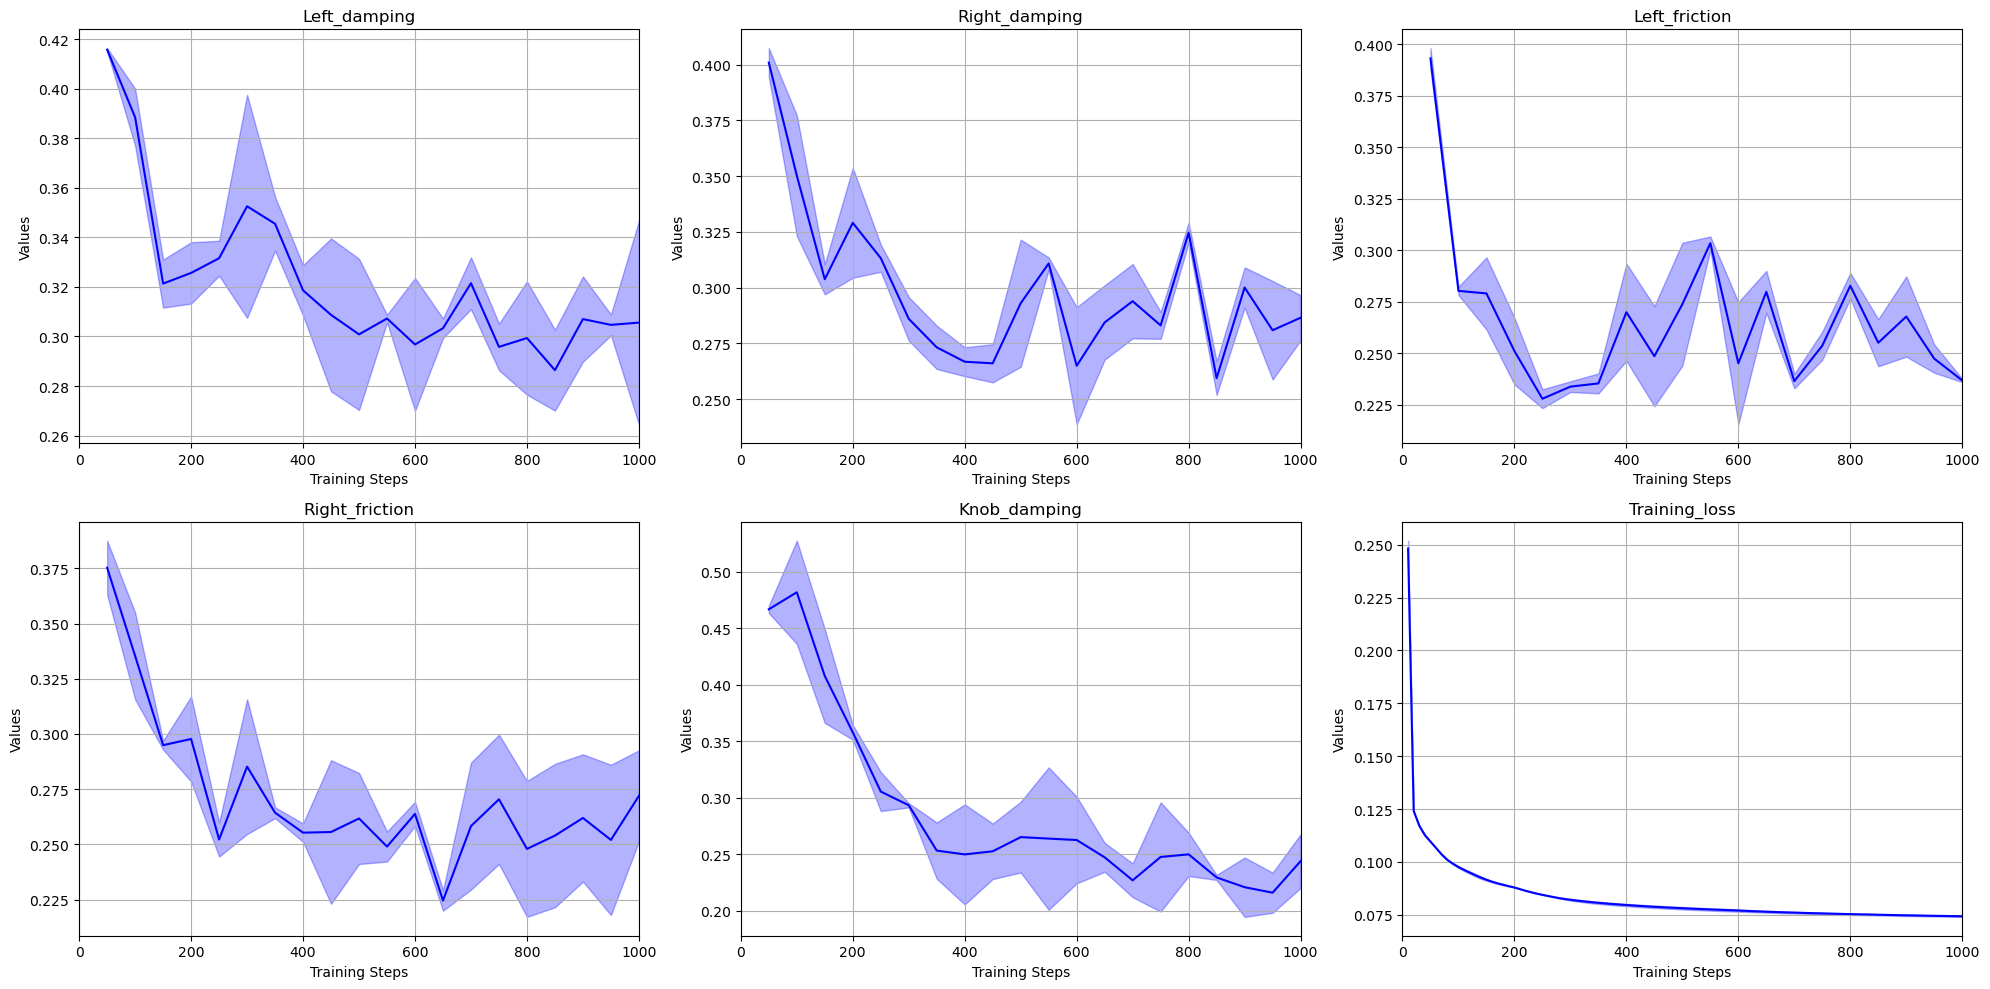}
            \caption{Training loss and evaluate results along the training process for table air hockey tasks.}
            \label{fig:traing_loss}
        \end{figure}
    \end{itemize}

\clearpage
\subsection*{Experiment 7: Evaluation with Noisy state observations}
\label{sec:exp_7}

    To further assess the robustness of CAPTURE, we explicitly evaluated the sim-to-sim transfer performance with added noise/perturbation. 
    \begin{itemize}
        \item \textbf{pose disturbance for object scooping:} Throughout our 30 adaptation iterations, we introduced a random angle label (from 0, -1, 1) every 3 steps to simulate disturbances. At each evaluation (30 adaptation iterations), 10 random labels were generated to act as noise for the angle classifier in the noisy setting. The results are evaluated in the sim-to-sim transfer with 100 randomly generated source-and-target pairs, shown in Figure~\ref{fig:scoop_noise}, reveal slight fluctuations in performance across adaptation iterations. Despite the high frequency of observation failures, CAPTURE consistently maintained robust performance and even outperformed baseline methods that utilized ground-truth state observations.

        \item \textbf{sensor noise for table air hockey:} In the table air hockey setting, randomly selecting state trajectories would not be a logical approach. Instead, we introduced uniform noise at each iteration to the real state trajectory component, resulting in observed real trajectory values ranging between 90\% and 110\% of the ground-truth values. As shown in Figure~\ref{fig:push_one_noise}, this significant noise slows down the adaptation process and slightly impacts performance. However, similar to the object scooping scenario, CAPTURE demonstrates resilience to noisy observations. By the later adaptation iterations, CAPTURE outperforms the baseline methods by a substantial margin, highlighting its robustness in noisy environments.

    \end{itemize}

    \begin{figure}[h]
        \centering
        \includegraphics[width=\linewidth]{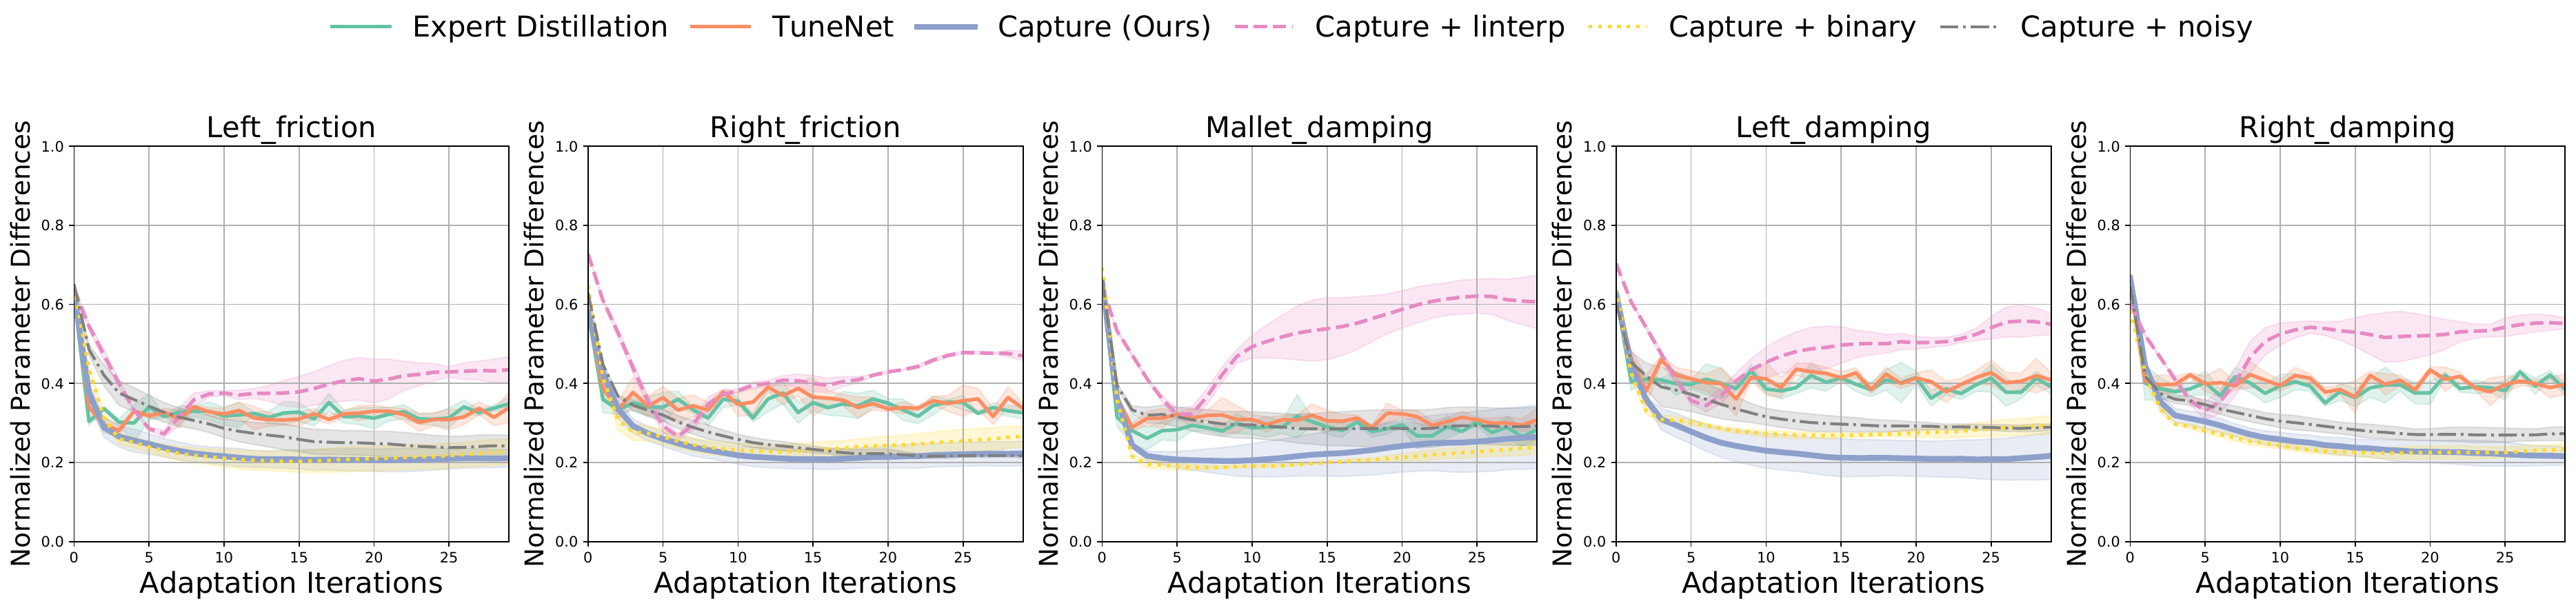}
        \caption{Table air hockey sim-to-sim transfer with noisy observations. }
        \label{fig:push_one_noise}
    \end{figure}
    \begin{figure}[h]
        \centering
        \includegraphics[width=0.7\linewidth]{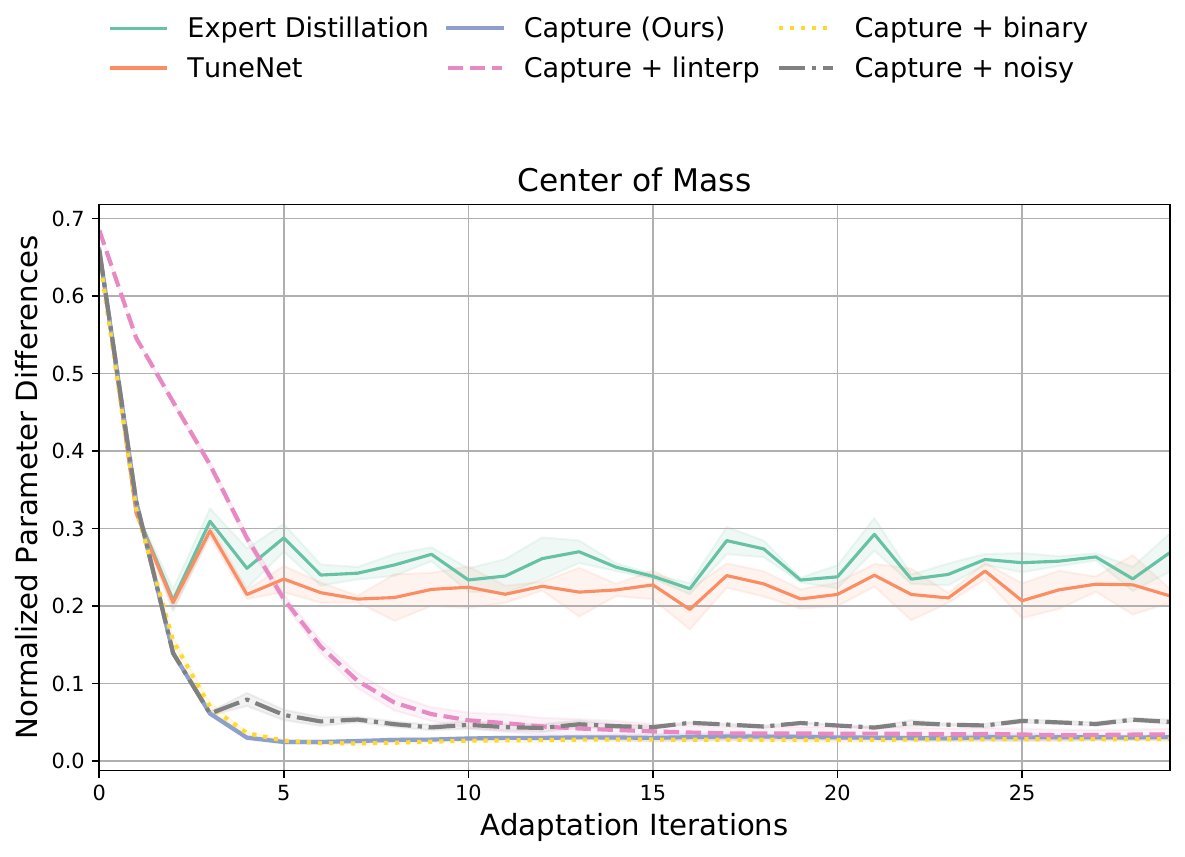}
        \caption{Object Scooping sim-to-sim transfer with noisy observations.}
        \label{fig:scoop_noise}
    \end{figure}
    
% \clearpage
% \subsection*{Experiment 8: Training curves}
% \label{sec:exp_8}

\end{document}
